# Supplementary material for: Learn-Explain-Reinforce: Counterfactual Reasoning and Its Guidance to Reinforce an Alzheimer's Disease Diagnosis Model
Source: arXiv:2108.09451 source file (2021-08-21)
Supplement: Supplementary file 1 [file supplementary.tex]

\setcounter{figure}{0}
\setcounter{table}{0}

\setcounter{section}{0}
%%%%%%%%%%%%%%%%%%%%%%%%%%%%%%%%%%%%%%%%%%%%%%%%%%%%%%%
\setcounter{page}{15} %15

\begin{center}\LARGE\bfseries
Supplementary Materials
\end{center}

% 1. Detailed Implementation
% % sup:1MNIST
% % sup:1ADNI
% 2. Details of the ADNI dataset
% % sup:2demo
% % sup:2long
% 3. Qualitative results (three classifier)
% % sup:3iter
% 4. Quantitative results
% % sup:4acc
% % sup:4ncc
% 5. Ablation Study
% % sup:5fid
% 6. Effectiveness of XGA module
% % sup:6effect

\section*{Section 1: Detailed Implementation}\label{sup1:implementation}
In each Table \ref{tab:mnist_g}, and \ref{tab:adni_g}, $(\cdot)^*$ denotes the skip-connection layer that passed through the convolution layer of three kernel size, one stride after concatenation with the tiled target condition. In the case of feature maps used in $(\cdot)^*$, we used the same number of feature maps of the counterfactual map generator to be concatenated. We performed $n$-D convolutional operation in the order of Conv.$\rightarrow$BatchNorm.$\rightarrow$Activation. We used a counterfactual map generator $\mathcal{G}_{\phi}$ that has the same network design as the encoder $\mathcal{E}_{\theta}$ with down-sampling layers replaced by up-sampling layers in all experiments.

\subsection*{Subsection 1.1: MNIST}\label{supsub1:mnist_net}
 The encoder network structure proposed by Kim \etal~\cite{kim2018disentangling} was utilized with minor modifications (\eg, in kernel and stride size). The discriminator network $\mathcal{D}_{\psi}$ is similar to the network design of the encoder $\mathcal{E}_{\theta}$, while the activation function in convolution layers and whether or not to use the normalization on certain layers was changed.
 
\label{sup:1MNIST}
\begin{table}[h]

\centering
\caption{MNIST encoder $\mathcal{E}_{\theta}$ network.}
\label{tab:encoder}
\begin{tabular}{@{}rlcccccl@{}}
\toprule
Operation & Feature Maps & Batch Norm. & Kernels & Strides & Padding & Activation &\\ \midrule

Input $\mathbf{X}\in\mathbb{R}^{28 \times 28 \times 1}$ &  &  &  &  &  &  \\
2D Conv. & \multicolumn{1}{c}{32} & $\surd$ & (3 $\times$ 3) & (1 $\times$ 1) & $\surd$ & \multicolumn{1}{c}{ReLU} \\
(ENC1) 2D Conv. & \multicolumn{1}{c}{32} & $\surd$ & (4 $\times$ 4) & (2 $\times$ 2) & $\surd$ & \multicolumn{1}{c}{ReLU} \\
2D Conv. & \multicolumn{1}{c}{64} & $\surd$ & (3 $\times$ 3) & (1 $\times$ 1) & $\surd$ & \multicolumn{1}{c}{ReLU} \\
(ENC2) 2D Conv. & \multicolumn{1}{c}{64} & $\surd$ & (4 $\times$ 4) & (2 $\times$ 2) & $\surd$ & \multicolumn{1}{c}{ReLU} \\
2D Conv. & \multicolumn{1}{c}{128} & $\surd$ & (3 $\times$ 3) & (1 $\times$ 1) & $\surd$ & \multicolumn{1}{c}{ReLU} \\
(ENC3) 2D Conv. & \multicolumn{1}{c}{128} & $\surd$ & (4 $\times$ 4) & (2 $\times$ 2) & $\surd$ & \multicolumn{1}{c}{ReLU} \\
2D Conv. & \multicolumn{1}{c}{256} & $\surd$ & (3 $\times$ 3) & (1 $\times$ 1) & $\surd$ & \multicolumn{1}{c}{ReLU} \\
(ENC4) 2D Conv. & \multicolumn{1}{c}{256} & $\surd$ & (4 $\times$ 4) & (2 $\times$ 2) & $\surd$ & \multicolumn{1}{c}{ReLU} \\
\bottomrule
\end{tabular}
\end{table}

\begin{table}[h]

\centering
\caption{MNIST classifier.}
\label{tab:encoder}
\begin{tabular}{@{}rlcccccl@{}}
\toprule
Operation & Feature Maps & Batch Norm. & Dropout & Activation &\\ \midrule
Input $\mathbf{X}\in\mathbb{R}^{2 \times 2 \times 256}$ &  &  &  &  &  &  \\
Fully Connected & \multicolumn{1}{c}{128} & $\times$ & 0.5 & \multicolumn{1}{c}{ReLU} \\
Fully Connected & \multicolumn{1}{c}{10} & $\times$ & 0.25 & \multicolumn{1}{c}{Softmax} \\

\bottomrule
\end{tabular}
\end{table}

\begin{table}[h]

\centering
\caption{MNIST discriminator $\mathcal{D}_{\psi}$ network.}
\label{tab:encoder}
\begin{tabular}{@{}rlcccccl@{}}
\toprule
Operation & Feature Maps & Batch Norm. & Kernels & Strides & Padding & Activation &\\ \midrule

Input $\mathbf{X}\in\mathbb{R}^{28 \times 28 \times 1}$ &  &  &  &  &  &  \\
2D Conv. & \multicolumn{1}{c}{32} & $\times$ & (3 $\times$ 3) & (1 $\times$ 1) & $\surd$ & \multicolumn{1}{c}{LReLU} \\
2D Conv. & \multicolumn{1}{c}{32} & $\surd$ & (4 $\times$ 4) & (2 $\times$ 2) & $\surd$ & \multicolumn{1}{c}{LReLU} \\
2D Conv. & \multicolumn{1}{c}{64} & $\surd$ & (3 $\times$ 3) & (1 $\times$ 1) & $\surd$ & \multicolumn{1}{c}{LReLU} \\
2D Conv. & \multicolumn{1}{c}{64} & $\surd$ & (4 $\times$ 4) & (2 $\times$ 2) & $\surd$ & \multicolumn{1}{c}{LReLU} \\
2D Conv. & \multicolumn{1}{c}{128} & $\surd$ & (3 $\times$ 3) & (1 $\times$ 1) & $\surd$ & \multicolumn{1}{c}{LReLU} \\
2D Conv. & \multicolumn{1}{c}{128} & $\surd$ & (4 $\times$ 4) & (2 $\times$ 2) & $\surd$ & \multicolumn{1}{c}{LReLU} \\
2D Conv. & \multicolumn{1}{c}{256} & $\surd$ & (3 $\times$ 3) & (1 $\times$ 1) & $\surd$ & \multicolumn{1}{c}{LReLU} \\
2D Conv. & \multicolumn{1}{c}{256} & $\surd$ & (4 $\times$ 4) & (2 $\times$ 2) & $\surd$ & \multicolumn{1}{c}{LReLU} \\
Fully Connected & \multicolumn{1}{c}{1} & $\times$ & & & & \multicolumn{1}{c}{Linear}\\
\bottomrule
\end{tabular}
\end{table}

\begin{table}[h]

\centering
\caption{MNIST counterfactual map generator $\mathcal{G}_{\phi}$ network.}
\label{tab:mnist_g}
\begin{tabular}{@{}rlcccccl@{}}
\toprule
Operation & Feature Maps & Batch Norm. & Kernels & Strides & Padding & Activation &\\ \midrule
Input $\mathbf{X}\in\mathbb{R}^{2 \times 2 \times 256}$ &  &  &  &  &  &  \\
Upsampling & & & & (2 $\times$ 2) & & \\
(DEC3) 2D Conv. & \multicolumn{1}{c}{128} & $\surd$ & (3 $\times$ 3) & (1 $\times$ 1) & $\surd$ & \multicolumn{1}{c}{ReLU}\\
\multicolumn{5}{c}{Concatenate $\text{(ENC3)}^*$ and (DEC3) along the channel axis} \\
2D Conv. & \multicolumn{1}{c}{128} & $\surd$ & (3 $\times$ 3) & (1 $\times$ 1) & $\surd$ & \multicolumn{1}{c}{ReLU}\\

Upsampling & & & & (2 $\times$ 2) & & \\
(DEC2) 2D Conv. & \multicolumn{1}{c}{64} & $\surd$ & (2 $\times$ 2) & (1 $\times$ 1) &  & \multicolumn{1}{c}{ReLU}\\
\multicolumn{5}{c}{Concatenate $\text{(ENC2)}^*$ and (DEC2) along the channel axis} \\
2D Conv. & \multicolumn{1}{c}{64} & $\surd$ & (3 $\times$ 3) & (1 $\times$ 1) & $\surd$ & \multicolumn{1}{c}{ReLU}\\

Upsampling & & & & (2 $\times$ 2) & & \\
(DEC1) 2D Conv. & \multicolumn{1}{c}{32} & $\surd$ & (3 $\times$ 3) & (1 $\times$ 1) & $\surd$ & \multicolumn{1}{c}{ReLU}\\
\multicolumn{5}{c}{Concatenate $\text{(ENC1)}^*$ and (DEC1) along the channel axis} \\
2D Conv. & \multicolumn{1}{c}{32} & $\surd$ & (3 $\times$ 3) & (1 $\times$ 1) & $\surd$ & \multicolumn{1}{c}{ReLU}\\
2D Deconv & \multicolumn{1}{c}{1} & $\surd$ & (4 $\times$ 4) & (2 $\times$ 2) & $\surd$ & \multicolumn{1}{c}{Tanh}\\

\bottomrule
\end{tabular}
\end{table}

\clearpage
\subsection*{Subsection 1.2: ADNI}\label{supsub1:adni_net}
 In ADNI experiment, the encoder network of ResNet18~\cite{he2016deep} was used identically and the counterfactual map generator $\mathcal{G}_{\phi}$ (\ie, decoder network) has the same network design as the encoder $\mathcal{E}_{\theta}$ with pooling layers replaced by up-sampling layers. We have utilized the encoder of SonoNet16~\cite{baumgartner2017sononet} as the discriminator network $\mathcal{D}_{\psi}$ via a minor modification (\eg, activation function) for all ADNI experiments.

% % DC architecutre 
% refer to the original paper

\begin{table}[h]

\centering
\caption{ADNI encoder $\mathcal{E}_{\theta}$ network.}
\label{tab:encoder}
\begin{tabular}{@{}rlccccccl@{}}
\toprule
Operation & Feature Maps & Batch Norm. & Kernels & Strides & Padding & Activation &\\ \midrule

Input $\mathbf{X}\in\mathbb{R}^{96 \times 114 \times 96 \times 1}$ &  &  &  &  &  &  &  \\
(ENC1) 3D Conv. & \multicolumn{1}{c}{64} & $\surd$ & (7 $\times$ 7 $\times$ 7) & (2 $\times$ 2 $\times$ 2) & $\surd$ & \multicolumn{1}{c}{ReLU} \\
% (ENC1) 3D Conv. & \multicolumn{1}{c}{64} & $\surd$ & (3 $\times$ 3 $\times$ 3) & (1 $\times$ 1 $\times$ 1) & $\surd$ & \multicolumn{1}{c}{ReLU} \\
Max pooling & & & (3 $\times$ 3 $\times$ 3) & (2 $\times$ 2 $\times$ 2) &  & \\

3D Conv. & \multicolumn{1}{c}{64} & $\surd$ & (3 $\times$ 3 $\times$ 3) & (1 $\times$ 1 $\times$ 1) & $\surd$ & \multicolumn{1}{c}{ReLU} \\
(ENC2) 3D Conv. & \multicolumn{1}{c}{64} & $\surd$ & (3 $\times$ 3 $\times$ 3) & (1 $\times$ 1 $\times$ 1) & $\surd$ & \multicolumn{1}{c}{ReLU} \\
Max pooling & & & (2 $\times$ 2 $\times$ 2) & (2 $\times$ 2 $\times$ 2) &  & \\

% 3D Conv. & \multicolumn{1}{c}{128} & $\surd$ & (3 $\times$ 3 $\times$ 3) & (1 $\times$ 1 $\times$ 1) & $\surd$ & \multicolumn{1}{c}{ReLU} \\
3D Conv. & \multicolumn{1}{c}{128} & $\surd$ & (3 $\times$ 3 $\times$ 3) & (1 $\times$ 1 $\times$ 1) & $\surd$ & \multicolumn{1}{c}{ReLU} \\
(ENC3) 3D Conv. & \multicolumn{1}{c}{128} & $\surd$ & (3 $\times$ 3 $\times$ 3) & (1 $\times$ 1 $\times$ 1) & $\surd$ & \multicolumn{1}{c}{ReLU} \\
Max pooling & & & (2 $\times$ 2 $\times$ 2) & (2 $\times$ 2 $\times$ 2) &  & \\

% 3D Conv. & \multicolumn{1}{c}{256} & $\surd$ & (3 $\times$ 3 $\times$ 3) & (1 $\times$ 1 $\times$ 1) & $\surd$ & \multicolumn{1}{c}{ReLU} \\
3D Conv. & \multicolumn{1}{c}{256} & $\surd$ & (3 $\times$ 3 $\times$ 3) & (1 $\times$ 1 $\times$ 1) & $\surd$ & \multicolumn{1}{c}{ReLU} \\
(ENC4) 3D Conv. & \multicolumn{1}{c}{256} & $\surd$ & (3 $\times$ 3 $\times$ 3) & (1 $\times$ 1 $\times$ 1) & $\surd$ & \multicolumn{1}{c}{ReLU} \\
Max pooling & & & (2 $\times$ 2 $\times$ 2) & (2 $\times$ 2 $\times$ 2) &  & \\

% 3D Conv. & \multicolumn{1}{c}{512} & $\surd$ & (3 $\times$ 3 $\times$ 3) & (1 $\times$ 1 $\times$ 1) & $\surd$ & \multicolumn{1}{c}{ReLU} \\
3D Conv. & \multicolumn{1}{c}{512} & $\surd$ & (3 $\times$ 3 $\times$ 3) & (1 $\times$ 1 $\times$ 1) & $\surd$ & \multicolumn{1}{c}{ReLU} \\
3D Conv. & \multicolumn{1}{c}{512} & $\surd$ & (3 $\times$ 3 $\times$ 3) & (1 $\times$ 1 $\times$ 1) & $\surd$ & \multicolumn{1}{c}{ReLU} \\
\bottomrule
\end{tabular}
\end{table}

\begin{table}[h]

\centering
\caption{ADNI classifier.}
\label{tab:encoder}
\begin{tabular}{@{}rlcccccl@{}}
\toprule
Operation & Feature Maps & Batch Norm. & Dropout & Activation &\\ \midrule
Input $\mathbf{X}\in\mathbb{R}^{3 \times 4 \times 3 \times 512}$ &  &  &  &  &  &  \\
Global Average Pooling & \multicolumn{1}{c}{512} & $\times$ & $\times$ & $\times$ \\
Fully Connected & \multicolumn{1}{c}{2} & $\times$ & $\times$ & \multicolumn{1}{c}{Softmax} \\

\bottomrule
\end{tabular}
\end{table}

\begin{table}[h]

\centering
\caption{ADNI discriminator $\mathcal{D}_{\psi}$ network.}
\label{tab:encoder}
\begin{tabular}{@{}rlcccccl@{}}
\toprule
Operation & Feature Maps & Batch Norm. & Kernels & Strides & Padding & Activation &\\ \midrule
Input $\mathbf{X}\in\mathbb{R}^{96 \times 114 \times 96 \times 1}$ &  &  &  &  &  &  \\
3D Conv. & \multicolumn{1}{c}{16} & $\times$ & (3 $\times$ 3 $\times$ 3) & (1 $\times$ 1 $\times$ 1) & $\surd$ & \multicolumn{1}{c}{LReLU} \\
3D Conv. & \multicolumn{1}{c}{16} & $\surd$ & (3 $\times$ 3 $\times$ 3) & (1 $\times$ 1$\times$ 1) & $\surd$ & \multicolumn{1}{c}{LReLU} \\
Max pooling & & & (2 $\times$ 2 $\times$ 2) & (2 $\times$ 2 $\times$ 2) &  &  \\

3D Conv. & \multicolumn{1}{c}{32} & $\surd$ & (3 $\times$ 3 $\times$ 3) & (1 $\times$ 1 $\times$ 1) & $\surd$ & \multicolumn{1}{c}{LReLU} \\
3D Conv. & \multicolumn{1}{c}{32} & $\surd$ & (3 $\times$ 3 $\times$ 3) & (1 $\times$ 1 $\times$ 1) & $\surd$ & \multicolumn{1}{c}{LReLU} \\
Max pooling & & & (2 $\times$ 2 $\times$ 2) & (2 $\times$ 2 $\times$ 2) &  & \\

3D Conv. & \multicolumn{1}{c}{64} & $\surd$ & (3 $\times$ 3 $\times$ 3) & (1 $\times$ 1 $\times$ 1) & $\surd$ & \multicolumn{1}{c}{LReLU} \\
3D Conv. & \multicolumn{1}{c}{64} & $\surd$ & (3 $\times$ 3 $\times$ 3) & (1 $\times$ 1 $\times$ 1) & $\surd$ & \multicolumn{1}{c}{LReLU} \\
3D Conv. & \multicolumn{1}{c}{64} & $\surd$ & (3 $\times$ 3 $\times$ 3) & (1 $\times$ 1 $\times$ 1) & $\surd$ & \multicolumn{1}{c}{LReLU} \\
Max pooling & & & (2 $\times$ 2 $\times$ 2) & (2 $\times$ 2 $\times$ 2) &  & \\

3D Conv. & \multicolumn{1}{c}{128} & $\surd$ & (3 $\times$ 3 $\times$ 3) & (1 $\times$ 1 $\times$ 1) & $\surd$ & \multicolumn{1}{c}{LReLU} \\
3D Conv. & \multicolumn{1}{c}{128} & $\surd$ & (3 $\times$ 3 $\times$ 3) & (1 $\times$ 1 $\times$ 1) & $\surd$ & \multicolumn{1}{c}{LReLU} \\
3D Conv. & \multicolumn{1}{c}{128} & $\surd$ & (3 $\times$ 3 $\times$ 3) & (1 $\times$ 1 $\times$ 1) & $\surd$ & \multicolumn{1}{c}{LReLU} \\
Max pooling & & & (2 $\times$ 2 $\times$ 2) & (2 $\times$ 2 $\times$ 2) &  & \\

3D Conv. & \multicolumn{1}{c}{128} & $\surd$ & (3 $\times$ 3 $\times$ 3) & (1 $\times$ 1 $\times$ 1) & $\surd$ & \multicolumn{1}{c}{LReLU} \\
3D Conv. & \multicolumn{1}{c}{128} & $\surd$ & (3 $\times$ 3 $\times$ 3) & (1 $\times$ 1 $\times$ 1) & $\surd$ & \multicolumn{1}{c}{LReLU} \\
3D Conv. & \multicolumn{1}{c}{128} & $\surd$ & (3 $\times$ 3 $\times$ 3) & (1 $\times$ 1 $\times$ 1) & $\surd$ &  \multicolumn{1}{c}{LReLU} \\
Fully Connected & \multicolumn{1}{c}{1} & $\times$ & & & & \multicolumn{1}{c}{Linear}\\
\bottomrule
\end{tabular}
\end{table}

\clearpage
\begin{table}[h]

\centering
\caption{ADNI counterfactual map generator $\mathcal{G}_{\phi}$ network.}
\label{tab:adni_g}
\begin{tabular}{@{}rlcccccl@{}}
\toprule
Operation & Feature Maps & Batch Norm. & Kernels & Strides & Padding & Activation &\\ \midrule
Input $\mathbf{X}\in\mathbb{R}^{3 \times 4 \times 3 \times 512}$ &  &  &  &  &  &  \\
\multicolumn{6}{c}{Concatenate Input $\mathbf{X}$ and tiled target condition along the channel axis} \\
% 3D Conv. & \multicolumn{1}{c}{512} & $\surd$ & (3 $\times$ 3 $\times$ 3) & (1 $\times$ 1 $\times$ 1) & $\surd$ & \multicolumn{1}{c}{LReLU}\\
3D Conv. & \multicolumn{1}{c}{512} & $\surd$ & (3 $\times$ 3 $\times$ 3) & (1 $\times$ 1 $\times$ 1) & $\surd$ & \multicolumn{1}{c}{LReLU}\\
(DEC4) Upsampling & & & & (2 $\times$ 2 $\times$ 2) & & \\
\multicolumn{5}{c}{Concatenate $\text{(ENC4)}^*$ and (DEC4) along the channel axis} \\
3D Conv. & \multicolumn{1}{c}{256} & $\surd$ & (3 $\times$ 3 $\times$ 3) & (1 $\times$ 1 $\times$ 1) & $\surd$ & \multicolumn{1}{c}{LReLU}\\
3D Conv. & \multicolumn{1}{c}{256} & $\surd$ & (3 $\times$ 3 $\times$ 3) & (1 $\times$ 1 $\times$ 1) & $\surd$ & \multicolumn{1}{c}{LReLU}\\

Upsampling & & & & (2 $\times$ 2 $\times$ 2) & & \\
(DEC3) 3D Deconv. & \multicolumn{1}{c}{128} & $\surd$ & (1 $\times$ 2 $\times$ 1) & (1 $\times$ 1 $\times$ 1) &  & \multicolumn{1}{c}{LReLU}\\
\multicolumn{5}{c}{Concatenate $\text{(ENC3)}^*$ and (DEC3) along the channel axis} \\
3D Conv. & \multicolumn{1}{c}{128} & $\surd$ & (3 $\times$ 3 $\times$ 3) & (1 $\times$ 1 $\times$ 1) & $\surd$ & \multicolumn{1}{c}{LReLU}\\
3D Conv. & \multicolumn{1}{c}{128} & $\surd$ & (3 $\times$ 3 $\times$ 3) & (1 $\times$ 1 $\times$ 1) & $\surd$ & \multicolumn{1}{c}{LReLU}\\

Upsampling & & & & (2 $\times$ 2 $\times$ 2) & & \\
(DEC2) 3D Deconv. & \multicolumn{1}{c}{64} & $\surd$ & (1 $\times$ 2 $\times$ 1) & (1 $\times$ 1 $\times$ 1) &  & \multicolumn{1}{c}{LReLU}\\
\multicolumn{5}{c}{Concatenate $\text{(ENC2)}^*$ and (DEC2) along the channel axis} \\
3D Conv. & \multicolumn{1}{c}{64} & $\surd$ & (3 $\times$ 3 $\times$ 3) & (1 $\times$ 1 $\times$ 1) & $\surd$ & \multicolumn{1}{c}{LReLU}\\
3D Conv. & \multicolumn{1}{c}{64} & $\surd$ & (3 $\times$ 3 $\times$ 3) & (1 $\times$ 1 $\times$ 1) & $\surd$ & \multicolumn{1}{c}{LReLU}\\

Upsampling & & & & (2 $\times$ 2 $\times$ 2) & & \\
(DEC1) 3D Deconv. & \multicolumn{1}{c}{64} & $\surd$ & (1 $\times$ 2 $\times$ 1) & (1 $\times$ 1 $\times$ 1) &  & \multicolumn{1}{c}{LReLU}\\
\multicolumn{5}{c}{Concatenate $\text{(ENC1)}^*$ and (DEC1) along the channel axis} \\
3D Conv. & \multicolumn{1}{c}{64} & $\surd$ & (3 $\times$ 3 $\times$ 3) & (1 $\times$ 1 $\times$ 1) & $\surd$ & \multicolumn{1}{c}{LReLU}\\
3D Conv. & \multicolumn{1}{c}{64} & $\surd$ & (3 $\times$ 3 $\times$ 3) & (1 $\times$ 1 $\times$ 1) & $\surd$ & \multicolumn{1}{c}{LReLU}\\
Upsampling & & & & (2 $\times$ 2 $\times$ 2) & & \\
3D Conv. & \multicolumn{1}{c}{1} & $\surd$ & (3 $\times$ 3 $\times$ 3) & (1 $\times$ 1 $\times$ 1) & $\surd$ & \multicolumn{1}{c}{Linear}\\
\bottomrule
\end{tabular}
\end{table}

\subsection*{Subsection 1.3: Hyperparameters}\label{supsub:1hyper}
The best performing model hyperparameters are shown below. $\lambda_{2,7}$ values are initialized to zero in the MNIST experiment given that $\ell_2$ normalization and total variation tend to soften the edges, which is beneficial for ADNI counterfactual maps but disadvantageous for images with hard edges. We exploited the same setting for the XGA module training in all scenarios (\ie, binary and multi-class classification).

\begin{table}[h]

\centering
\caption{MNIST model hyperparameters for the classifier.}
\label{tab:omni-hyper}
\begin{tabular}{@{}rlccl@{}}
\toprule
Epochs $\&$ Batch Size & \multicolumn{4}{l}{50, 128}\\
Optimizer & \multicolumn{4}{l}{Adam $\left(\beta_1=0.9, \beta_2=0.999\right)$} \\
% Learning $\&$ Exponential Decay Rate  & \multicolumn{4}{l}{0.0005, 0.98}\\
Learning Rate  & \multicolumn{4}{l}{0.0005}\\
Exponential Decay Rate  & \multicolumn{4}{l}{0.98}\\
\bottomrule
\end{tabular}
\end{table}

\begin{table}[h]

\centering
\caption{MNIST model hyperparameters for the counterfactual map generation.}
\label{tab:omni-hyper}
\begin{tabular}{@{}rlccl@{}}
\toprule
Epochs $\&$ Batch Size & \multicolumn{4}{l}{100, 128}\\
Optimizer & \multicolumn{4}{l}{Adam $\left(\beta_1=0.9, \beta_2=0.999\right)$} \\
One-sided Label Smoothing & \multicolumn{4}{l}{0.1}\\
% Learning $\&$ Exponential Decay Rate & \multicolumn{4}{l}{$\mathcal{G}_{\phi},\mathcal{D}_{\psi}$ = 0.001, 0.98}\\
Learning Rate & \multicolumn{4}{l}{$\mathcal{G}_{\phi},\mathcal{D}_{\psi}$ = 0.001}\\
Exponential Decay Rate & \multicolumn{4}{l}{0.98}\\
Weight Constants & \multicolumn{4}{l}{$\lambda_1=1, \lambda_2=0, \lambda_3=10, \lambda_4=1, \lambda_5=1, \lambda_6=1, \lambda_7=0$} \\
\bottomrule
\end{tabular}
\end{table}

\begin{table}[h]

\centering
\caption{ADNI model hyperparameters for the diagnostic model and XGA module training.}
\label{tab:omni-hyper}
\begin{tabular}{@{}rlccl@{}}
\toprule
Epochs $\&$ Batch Size & \multicolumn{4}{l}{150, 12}\\
Optimizer & \multicolumn{4}{l}{Adam $\left(\beta_1=0.9, \beta_2=0.999\right)$} \\
% Learning $\&$ Exponential Decay Rate & \multicolumn{4}{l}{0.0001, 0.98}\\
Learning Rate & \multicolumn{4}{l}{0.0001}\\
Exponential Decay Rate & \multicolumn{4}{l}{0.98}\\
Weight Constants $\&$ $r$ Rate  & \multicolumn{4}{l}{$\lambda_8=0.1$, 4 $(\text{excluded from the diagnostic model training})$} \\
\bottomrule
\end{tabular}
\end{table}

\begin{table}[!htbp]

\centering
\caption{ADNI model hyperparameters for the counterfactual map generation.}
\label{tab:omni-hyper}
\begin{tabular}{@{}rlccl@{}}
\toprule
Epochs $\&$ Batch Size & \multicolumn{4}{l}{100, 3}\\
Optimizer & \multicolumn{4}{l}{Adam $\left(\beta_1=0.9, \beta_2=0.999\right)$} \\
% Learning $\&$ Exponential Decay Rate & \multicolumn{4}{l}{$\mathcal{G}_{\phi},\mathcal{D}_{\psi}$ = 0.01, 1.0}\\
Learning Rate & \multicolumn{4}{l}{$\mathcal{G}_{\phi},\mathcal{D}_{\psi}$ = 0.01}\\
Exponential Decay Rate & \multicolumn{4}{l}{1.0}\\
Weight Constants & \multicolumn{4}{l}{$\lambda_1=10, \lambda_2=10, \lambda_3=10, \lambda_4=5, \lambda_5=1, \lambda_6=1, \lambda_7=5e^{-6}$} \\
\bottomrule
\end{tabular}
\end{table}

\clearpage
\section*{Section 2: Data Description of ADNI experiment}\label{sup:2data}
\subsection*{Subsection 2.1: Details of ADNI Dataset}\label{supsub:2data}
We used 431 CN subjects, 497 stable mild cognitive impairment (sMCI), 251 progressive mild cognitive impairment (pMCI), and 359 AD subjects in ADNI-1 and ADNI-2 studies. Thus, a total of 1,538 images were used in our experiments. For three-class experiments, sMCI and pMCI subjects were considered as MCI subjects. The gender was represented as male/female and the age, education, and MMSE scores were reported in terms of Mean $\pm$ Standard deviation (Std).

The pre-processing procedure consisted of neck removal (FSL v6.0.1 robustfov), brain extraction (HDBet~\cite{https://doi.org/10.1002/hbm.24750}), linear registration (FSL v6.0.1 FLIRT), zero-mean unit-variance normalization, quantile normalization at 10\% and 90\%, and down-scaling by $2\times$. The resulting pre-processed MRI is a $96 \times 114 \times 96$ image. We used the default parameters from FSL v6.0.1~\cite{JENKINSON2012782}.

\begin{table}[h]\scriptsize\setlength{\tabcolsep}{7.pt}
    \caption{Details of the demographic information of ADNI dataset.}
    \label{table:demegraphic information}
    \centering
    \begin{tabular}{cccccc}
    \toprule
    \multicolumn{1}{c}{\textbf{Dataset}} & \multicolumn{1}{c}{\textbf{Category}} & \multicolumn{1}{c}{\textbf{Gender}} & \multicolumn{1}{c}{\textbf{Age}} & \multicolumn{1}{c}{\textbf{Education}} & \multicolumn{1}{c}{\textbf{MMSE}}\\
\midrule
    \multicolumn{1}{c}{\multirow{4}{*}{ADNI-1}} & \multicolumn{1}{c}{CN} & \multicolumn{1}{c}{119/112} &\multicolumn{1}{c}{76.0$\pm$5.0} &\multicolumn{1}{c}{16.1$\pm$2.8} &\multicolumn{1}{c}{29.1$\pm$1.0} \\
     & \multicolumn{1}{c}{sMCI} & \multicolumn{1}{c}{148/75} &\multicolumn{1}{c}{74.8$\pm$7.7} &\multicolumn{1}{c}{15.5$\pm$3.2} &\multicolumn{1}{c}{27.3$\pm$1.8} \\
     & \multicolumn{1}{c}{pMCI} & \multicolumn{1}{c}{103/65} &\multicolumn{1}{c}{74.7$\pm$7.0} &\multicolumn{1}{c}{15.7$\pm$2.8} &\multicolumn{1}{c}{26.6$\pm$1.7} \\
     & \multicolumn{1}{c}{AD} & \multicolumn{1}{c}{103/97} &\multicolumn{1}{c}{75.6$\pm$7.7} &\multicolumn{1}{c}{14.7$\pm$3.2} &\multicolumn{1}{c}{23.3$\pm$2.0} \\
\midrule
    \multicolumn{1}{c}{\multirow{4}{*}{ADNI-2}} & \multicolumn{1}{c}{CN} & \multicolumn{1}{c}{97/107} &\multicolumn{1}{c}{73.4$\pm$6.4} &\multicolumn{1}{c}{16.6$\pm$2.5} &\multicolumn{1}{c}{29.0$\pm$1.2} \\
     & \multicolumn{1}{c}{sMCI} & \multicolumn{1}{c}{151/123} &\multicolumn{1}{c}{71.3$\pm$7.5} &\multicolumn{1}{c}{16.3$\pm$2.6} &\multicolumn{1}{c}{28.2$\pm$1.6} \\
     & \multicolumn{1}{c}{pMCI} & \multicolumn{1}{c}{45/38} &\multicolumn{1}{c}{72.9$\pm$7.2} &\multicolumn{1}{c}{16.2$\pm$2.3} &\multicolumn{1}{c}{27.1$\pm$1.8} \\
     & \multicolumn{1}{c}{AD} & \multicolumn{1}{c}{91/68} &\multicolumn{1}{c}{74.9$\pm$8.1} &\multicolumn{1}{c}{15.7$\pm$2.7} &\multicolumn{1}{c}{23.1$\pm$2.1} \\
\bottomrule
\end{tabular}
\end{table}

\subsection*{Subsection 2.2: Details of Longitudinal Dataset}\label{supsub:2long}
% Since there are no ground-truth maps for ADNI dataset~\cite{MUELLER2005869}, we utilized the ground-truth map from longitudinal test subjects. 
We produced ground-truth for counterfactual maps using MRIs from longitudinal subjects.
First, we gathered MRIs from 12 subjects who converted from CN (baseline) to MCI and AD at any later time point. Details of the subject ID with regard to each subject and image ID corresponding to CN, MCI, and AD are presented in Table~\ref{tab:adni_longitudinal_table}.
Then, to create the ground-truth map, we subtracted the target (AD) image from the baseline (CN) image. This ground-truth map exhibited a good representation of disease localization as it indicates which regions were changed along with the clinical label conversion.

The resulting ground-truth map and CF map of comparing visual explanation methods are overlaid onto a subject's sMRI in Fig.~\ref{fig:Brain_result}. 
As the ground-truth map in this figure is for CN←AD CF maps (\ie, ground-truth map = Image \#27607 (CN) - Image \#396124 (AD)), the positive (\ie, red color) regions should indicate, for example, reduced ventricular (purple boxes), increased cortical thickness (green boxes), and hypertrophy (as opposite to atrophy) in hippocampus regions (orange boxes).

\begin{table}[h]

\centering
\caption{ADNI longitudinal subject information for the quantitative evaluation of counterfactual map.}
\label{tab:adni_longitudinal_table}
\begin{tabular}{cccc}
\toprule
\multicolumn{1}{c}{\multirow{2}{*}{\textbf{Subject ID}}} & \multicolumn{1}{c}{\textbf{Cognitive normal (CN)}} & \multicolumn{1}{c}{\textbf{Mild cognitive impairment (MCI)}} & \multicolumn{1}{c}{\textbf{Alzheimer's disease (AD)}}\\
% \cmidrule(lr){3} \cmidrule(lr){4} \cmidrule(lr){5}
& \text{Image ID} & \text{Image ID} & \text{Image ID} \\
\cmidrule(lr){1-4}
$023\_\text{S}\_0061$ & 9046 & 401795 & 473765 \\
$123\_\text{S}\_0106$ & 10126 & 213947 & 865961 \\
$131\_\text{S}\_0123$ & 10042 & 292389 & 475755 \\
% $114\_\text{S}\_0166$ & 11018 & 289125 & 416112 \\
$005\_\text{S}\_0223$ & 11645 & 26115 & 143296 \\
$037\_\text{S}\_0467$ & 14861 & 169074 & 372375 \\
$129\_\text{S}\_0778$ & 20543 & 205611 & 388698 \\
$024\_\text{S}\_0985$ & 27607 & 342890 & 396124 \\
$023\_\text{S}\_1190$ & 35585 & 780686 & 1135165 \\
$002\_\text{S}\_4262$ & 259653 & 397601 & 788894 \\
$029\_\text{S}\_4385$ & 285589 & 421501 & 642470 \\
$098\_\text{S}\_4506$ & 286987 & 714545 & 1073489 \\
$051\_\text{S}\_5285$ & 396288 & 1055626 & 1182436 \\
\bottomrule
\end{tabular}
\end{table}

%%%%%%%%%%%%%%%%%%%%%%%%%%%%%%%%%%%%%%%%%%%%%%%%%%%%%%%
\clearpage
\section*{Section 3: Quantitative Results of the binary scenarios on ADNI}\label{sup:3res}
\subsection*{Subsection 3.1: Quantitative results with XGA module applied to conventional CNN-based methods}\label{supsub:3ncc}
% To validate the generalizability and effectiveness of our proposed XGA module, we applied this module in various diagnostic models. 

\begin{table}[h]\scriptsize \setlength{\tabcolsep}{3.pt}
    \caption{Normalized cross-correlation (NCC) scores with the XGA module utilized to various diagnostic models.}
    \centering
    \label{tab:compared_exp2}
    \begin{tabular}{ccccccc}
    \toprule
    \multicolumn{1}{c}{\multirow{2}{*}{\textbf{Scenario}}} & \multicolumn{2}{c}{\textbf{CN $\leftrightarrow$ MCI}} & \multicolumn{2}{c}{\textbf{MCI $\leftrightarrow$ AD}} & \multicolumn{2}{c}{\textbf{CN $\leftrightarrow$ AD}}\\
    \cmidrule(lr){2-3} \cmidrule(lr){4-5} \cmidrule(lr){6-7}
    & \textbf{NCC(+)} & \textbf{NCC(-)} & \textbf{NCC(+)} & \textbf{NCC(-)} & \textbf{NCC(+)} & \textbf{NCC(-)}\\

\midrule
    \text{ResNet18/2-class} &\multicolumn{1}{c}{0.378} &\multicolumn{1}{c}{0.283} &\multicolumn{1}{c}{\bf{0.338}} &\multicolumn{1}{c}{0.289} &\multicolumn{1}{c}{0.378} &\multicolumn{1}{c}{0.306}\\
    \text{SonoNet16/2-class} &\multicolumn{1}{c}{\bf{0.401}} &\multicolumn{1}{c}{\bf{0.336}} &\multicolumn{1}{c}{0.323} &\multicolumn{1}{c}{\bf{0.351}} &\multicolumn{1}{c}{\bf{0.402}} &\multicolumn{1}{c}{\bf{0.368}}\\ 
    \text{VoxCNN/2-class} &\multicolumn{1}{c}{0.376} &\multicolumn{1}{c}{0.302} &\multicolumn{1}{c}{0.321} &\multicolumn{1}{c}{0.297} &\multicolumn{1}{c}{0.361} &\multicolumn{1}{c}{0.333}\\
    \midrule
    \text{ResNet18/3-class} &\multicolumn{1}{c}{0.364} &\multicolumn{1}{c}{0.289} &\multicolumn{1}{c}{0.299} &\multicolumn{1}{c}{0.297} &\multicolumn{1}{c}{0.366} &\multicolumn{1}{c}{0.312}\\
    \text{SonoNet16/3-class} &\multicolumn{1}{c}{\bf{0.388}} &\multicolumn{1}{c}{0.285} &\multicolumn{1}{c}{\bf{0.301}} &\multicolumn{1}{c}{\bf{0.364}} &\multicolumn{1}{c}{\bf{0.378}} &\multicolumn{1}{c}{0.306}\\ 
    \text{VoxCNN/3-class} &\multicolumn{1}{c}{0.363} &\multicolumn{1}{c}{\bf{0.300}} &\multicolumn{1}{c}{0.289} &\multicolumn{1}{c}{0.215} &\multicolumn{1}{c}{0.403} &\multicolumn{1}{c}{\bf{0.346}}\\ 
\bottomrule
\end{tabular}
\end{table}

\subsection*{Subsection 3.2: Binary classification results compared to recent studies}\label{supsub:3acc}
\begin{table*}[h]\scriptsize \setlength{\tabcolsep}{7.pt}
    \caption{Classification results of various binary scenarios on ADNI dataset.}
    \label{table:2cls_res}
    \centering
    \begin{tabular}{ccccccc}
    \toprule
         & \textbf{Guidance}& \textbf{Models} &\textbf{AUC} &\textbf{ACC} &\textbf{SEN} &\textbf{SPE}\\ 
        \cmidrule(lr){2-2}\cmidrule(lr){3-3} \cmidrule(lr){4-7}
        
        \parbox[t]{2mm}{\multirow{10}{*}{\rotatebox[origin=c]{90}{CN vs. MCI}}} &  & \multicolumn{1}{c}{ResNet18~\cite{he2016deep}} & \text{0.6209} $\pm$ \text{0.056} &\text{0.6479} $\pm$ \text{0.037} & \text{0.7487} $\pm$ \text{0.146} & \text{0.4931} $\pm$ \text{0.218} \\
        && \multicolumn{1}{c}{SonoNet16~\cite{baumgartner2017sononet}} & \text{0.6166} $\pm$ \text{0.027} & \text{0.6445} $\pm$ \text{0.042} & \text{0.7216} $\pm$ \text{0.174} & \text{0.5117} $\pm$ \text{0.202} \\
        && \multicolumn{1}{c}{VoxCNN~\cite{korolev2017residual}} & \text{0.5802} $\pm$ \text{0.047} & \text{0.6428} $\pm$ \text{0.035} & \text{0.8162} $\pm$ \text{0.108} & \text{0.3442} $\pm$ \text{0.171} \\
        && \multicolumn{1}{c}{Liu \etal~\cite{liu2020design}} & \text{0.5458} $\pm$ \text{0.043} & \text{0.6325} $\pm$ \text{0.024} & \text{0.8723} $\pm$ \text{0.083} & \text{0.2186} $\pm$ \text{0.153} \\
        && \multicolumn{1}{c}{Jin \etal~\cite{jin2019attention}} & \text{0.5914} $\pm$ \text{0.031} & \text{0.6359} $\pm$ \text{0.021} & \text{0.7595} $\pm$ \text{0.063} & \text{0.4233} $\pm$ \text{0.108} \\
        % && \multicolumn{1}{c}{Zhang \etal~\cite{zhang2021explainable}} & \text{-} $\pm$ \text{-} & \text{-} $\pm$ \text{-} & \text{-} $\pm$ \text{-} & \text{-} $\pm$ \text{-} \\
        
        \cmidrule(lr){2-7}
        & \hspace{0.cm}\parbox[t]{2mm}{\multirow{5}{*}{\rotatebox[origin=c]{0}{$\checkmark$}}} & \multicolumn{1}{c}{Li \etal~\cite{li2019novel}} & \text{0.6726} $\pm$ \text{0.033} & \text{0.6923} $\pm$ \text{0.041} & \text{0.8649} $\pm$ \text{0.077} & \text{0.4186} $\pm$ \text{0.168}  \\
        &  & \multicolumn{1}{c}{Lian \etal~\cite{lian2020attention}} & \text{0.6311} $\pm$ \text{0.048} & \text{0.6418} $\pm$ \text{0.027} & \text{0.8378} $\pm$ \text{0.082} & \text{0.4242} $\pm$ \text{0.178}\\
        && \multicolumn{1}{c}{\textbf{Ours (ResNet18 + XGA)}} & \text{0.6804} $\pm$ \text{0.053} &\text{0.7436} $\pm$ \text{0.042} & \text{0.9189} $\pm$ \text{0.067} & \text{0.4419} $\pm$ \text{0.066} \\
        && \multicolumn{1}{c}{\textbf{Ours (SonoNet16 + XGA)}} & \textbf{0.7404} $\pm$ \textbf{0.023} &\textbf{0.7641} $\pm$ \textbf{0.021} & \textbf{0.9459} $\pm$ \textbf{0.057} & \textbf{0.5349} $\pm$ \textbf{0.048} \\
        && \multicolumn{1}{c}{\textbf{Ours (VoxCNN + XGA)}} & \text{0.6882} $\pm$ \text{0.048} &\text{0.7161} $\pm$ \text{0.077} & \text{0.8984} $\pm$ \text{0.089} & \text{0.4879} $\pm$ \text{0.082} \\
        
        \cmidrule(lr){1-7}
        
        \parbox[t]{2mm}{\multirow{11}{*}{\rotatebox[origin=c]{90}{sMCI vs. pMCI}}} &  & \multicolumn{1}{c}{ResNet18~\cite{he2016deep}} & \text{0.6499} $\pm$ \text{0.054} &\text{0.6946} $\pm$ \text{0.051} & \text{0.5120} $\pm$ \text{0.158} & \text{0.7878} $\pm$ \text{0.114} \\
        & & \multicolumn{1}{c}{SonoNet16~\cite{baumgartner2017sononet}} & \text{0.6283} $\pm$ \text{0.066} & \text{0.6919} $\pm$ \text{0.048} & \text{0.4320} $\pm$ \text{0.196} & \text{0.8245} $\pm$ \text{0.111} \\
        && \multicolumn{1}{c}{VoxCNN~\cite{korolev2017residual}} & \text{0.6226} $\pm$ \text{0.081} & \text{0.6973} $\pm$ \text{0.037} & \text{0.3920} $\pm$ \text{0.247} & \text{0.8531} $\pm$ \text{0.104} \\
        && \multicolumn{1}{c}{Liu \etal~\cite{liu2020design}} & \text{0.6249} $\pm$ \text{0.043} & \text{0.7108} $\pm$ \text{0.036} & \text{0.3600} $\pm$ \text{0.123} & \text{0.8898} $\pm$ \text{0.079} \\
        && \multicolumn{1}{c}{Jin \etal~\cite{jin2019attention}} & \text{0.6234} $\pm$ \text{0.041} & \text{0.6595} $\pm$ \text{0.046} & \text{0.5120} $\pm$ \text{0.156} & \text{0.7347} $\pm$ \text{0.125} \\
        % && \multicolumn{1}{c}{Zhang \etal~\cite{zhang2021explainable}} & \text{-} $\pm$ \text{-} & \text{-} $\pm$ \text{-} & \text{-} $\pm$ \text{-} & \text{-} $\pm$ \text{-} \\

        \cmidrule(lr){2-7}
        & \hspace{0.cm}\parbox[t]{2mm}{\multirow{5}{*}{\rotatebox[origin=c]{0}{$\checkmark$}}} & \multicolumn{1}{c}{Li \etal~\cite{li2019novel}} & \text{0.6681} $\pm$ \text{0.045} & \text{0.7112} $\pm$ \text{0.052} & \text{0.4265} $\pm$ \text{0.128} & \text{0.8884} $\pm$ \text{0.091} \\
        &  & \multicolumn{1}{c}{Lian \etal~\cite{lian2020attention}} & \text{0.6683} $\pm$ \text{0.034} & \text{0.7031} $\pm$ \text{0.031} & \text{0.4106} $\pm$ \text{0.153} & \text{0.8511} $\pm$ \text{0.059}\\
        && \multicolumn{1}{c}{\textbf{Ours (ResNet18 + XGA)}} & \textbf{0.7469} $\pm$ \textbf{0.068} &\textbf{0.7703} $\pm$ \textbf{0.053} & \textbf{0.5201} $\pm$ \textbf{0.099} & \text{0.8981} $\pm$ \text{0.079} \\
        && \multicolumn{1}{c}{\textbf{Ours (SonoNet16 + XGA)}} & \text{0.7437} $\pm$ \text{0.058} &\text{0.7568} $\pm$ \text{0.044} & \text{0.4400} $\pm$ \text{0.123} & \textbf{0.9184} $\pm$ \textbf{0.104} \\
        && \multicolumn{1}{c}{\textbf{Ours (VoxCNN + XGA)}} & \text{0.7371} $\pm$ \text{0.072} &\text{0.7568} $\pm$ \text{0.034} & \text{0.4811} $\pm$ \text{0.183} & \textbf{0.8981} $\pm$ \textbf{0.068} \\
        
        \cmidrule(lr){1-7}
        
        \parbox[t]{2mm}{\multirow{11}{*}{\rotatebox[origin=c]{90}{MCI vs. AD}}} &  & \multicolumn{1}{c}{ResNet18~\cite{he2016deep}} & \text{0.7696} $\pm$ \text{0.087} &\text{0.7965} $\pm$ \text{0.065} & \text{0.6943} $\pm$ \text{0.091} & \text{0.8449} $\pm$ \text{0.083} \\
        & & \multicolumn{1}{c}{SonoNet16~\cite{baumgartner2017sononet}} & \text{0.6922} $\pm$ \text{0.032} & \text{0.7743} $\pm$ \text{0.024} & \text{0.4629} $\pm$ \text{0.064} & \text{0.9216} $\pm$ \text{0.085} \\
        && \multicolumn{1}{c}{VoxCNN~\cite{korolev2017residual}} & \text{0.7118} $\pm$ \text{0.086} & \text{0.7685} $\pm$ \text{0.036} & \text{0.5588} $\pm$ \text{0.276} & \text{0.8649} $\pm$ \text{0.053} \\
        && \multicolumn{1}{c}{Liu \etal~\cite{liu2020design}} & \text{0.6959} $\pm$ \text{0.078} & \text{0.7685} $\pm$ \text{0.061} & \text{0.581} $\pm$ \text{0.161} & \text{0.8919} $\pm$ \text{0.038} \\
        && \multicolumn{1}{c}{Jin \etal~\cite{jin2019attention}} & \text{0.7663} $\pm$ \text{0.115} & \text{0.7778} $\pm$ \text{0.051} & \text{0.7353} $\pm$ \text{0.195} & \text{0.7973} $\pm$ \text{0.079} \\
        % && \multicolumn{1}{c}{Zhang \etal~\cite{zhang2021explainable}} & \text{-} $\pm$ \text{-} & \text{-} $\pm$ \text{-} & \text{-} $\pm$ \text{-} & \text{-} $\pm$ \text{-} \\

        \cmidrule(lr){2-7}
        & \hspace{0.cm}\parbox[t]{2mm}{\multirow{5}{*}{\rotatebox[origin=c]{0}{$\checkmark$}}} & \multicolumn{1}{c}{Li \etal~\cite{li2019novel}} & \text{0.8104} $\pm$ \text{0.071} & \text{0.8056} $\pm$ \text{0.023} & \text{0.8235} $\pm$ \text{0.058} & \text{0.7973} $\pm$ \text{0.081} \\
        &  & \multicolumn{1}{c}{Lian \etal~\cite{lian2020attention}} & \text{0.7547} $\pm$ \text{0.008} & \text{0.7221} $\pm$ \text{0.019} & \text{0.6759} $\pm$ \text{0.114} & \text{0.9054} $\pm$ \text{0.094}\\
        && \multicolumn{1}{c}{\textbf{Ours (ResNet18 + XGA)}} & \textbf{0.8376} $\pm$ \textbf{0.036} &\textbf{0.8716} $\pm$ \textbf{0.048} & \textbf{0.7429} $\pm$ \textbf{0.064} & \text{0.9324} $\pm$ \text{0.035} \\
        && \multicolumn{1}{c}{\textbf{Ours (SonoNet16 + XGA)}} & \text{0.8048} $\pm$ \text{0.024} &\text{0.8441} $\pm$ \text{0.067} & \text{0.6671} $\pm$ \text{0.065} & \textbf{0.9424} $\pm$ \textbf{0.082} \\
        && \multicolumn{1}{c}{\textbf{Ours (VoxCNN + XGA)}} & \text{0.8086} $\pm$ \text{0.045} &\text{0.8581} $\pm$ \text{0.052} & \text{0.6992} $\pm$ \text{0.048} & \text{0.9184} $\pm$ \text{0.055} \\
        
        \cmidrule(lr){1-7}
        
        \parbox[t]{2mm}{\multirow{11}{*}{\rotatebox[origin=c]{90}{CN vs. AD}}} &  & \multicolumn{1}{c}{ResNet18~\cite{he2016deep}} & \text{0.8878} $\pm$ \text{0.036} &\text{0.8898} $\pm$ \text{0.036} & \text{0.8686} $\pm$ \text{0.043} & \text{0.9070} $\pm$ \text{0.055} \\
        &  & \multicolumn{1}{c}{SonoNet16~\cite{baumgartner2017sononet}} & \text{0.8897} $\pm$ \text{0.021} &\text{0.9077} $\pm$ \text{0.019} & \text{0.8400} $\pm$ \text{0.048} & \text{0.9395} $\pm$ \text{0.027} \\
        && \multicolumn{1}{c}{VoxCNN~\cite{korolev2017residual}} & \text{0.8663} $\pm$ \text{0.042} &\text{0.8667} $\pm$ \text{0.043} & \text{0.8629} $\pm$ \text{0.042} & \text{0.8698} $\pm$ \text{0.058} \\
        && \multicolumn{1}{c}{Liu \etal~\cite{liu2020design}} & \text{0.8308} $\pm$ \text{0.038} &\text{0.8333} $\pm$ \text{0.040} & \text{0.8057} $\pm$ \text{0.102} & \text{0.8558} $\pm$ \text{0.107} \\
        && \multicolumn{1}{c}{Jin \etal~\cite{jin2019attention}} & \text{0.8653} $\pm$ \text{0.041} &\text{0.8667} $\pm$ \text{0.041} & \text{0.8514} $\pm$ \text{0.051} & \text{0.8791} $\pm$ \text{0.058} \\
        % && \multicolumn{1}{c}{Zhang \etal~\cite{zhang2021explainable}} & \text{-} $\pm$ \text{-} & \text{-} $\pm$ \text{-} & \text{-} $\pm$ \text{-} & \text{-} $\pm$ \text{-} \\
        
        \cmidrule(lr){2-7}
        & \hspace{0.cm}\parbox[t]{2mm}{\multirow{5}{*}{\rotatebox[origin=c]{0}{$\checkmark$}}} & \multicolumn{1}{c}{Li \etal~\cite{li2019novel}} & \text{0.9209} $\pm$ \text{0.014} & \text{0.9231} $\pm$ \text{0.018} & \text{0.9000} $\pm$ \text{0.021} & \text{0.9418} $\pm$ \text{0.049}  \\
        &  & \multicolumn{1}{c}{Lian \etal~\cite{lian2020attention}} & \text{0.8995} $\pm$ \text {0.018} & \text{0.9039} $\pm$ \text{0.023} & \text{0.8429} $\pm$ \text{0.021} & \text{0.9418} $\pm$ \text{0.026}\\
        
        && \multicolumn{1}{c}{\textbf{Ours (ResNet18 + XGA)}} & \textbf{0.9498} $\pm$ \textbf{0.031} &\textbf{0.9515} $\pm$ \textbf{0.038} & \textbf{0.9429} $\pm$ \textbf{0.041} & \textbf{0.9667} $\pm$ \textbf{0.082} \\
        && \multicolumn{1}{c}{\textbf{Ours (SonoNet16 + XGA)}} & \text{0.9339} $\pm$ \text{0.016} &\text{0.9359} $\pm$ \text{0.016} & \text{0.9143} $\pm$ \text{0.037} & \text{0.9535} $\pm$ \text{0.031} \\
        && \multicolumn{1}{c}{\textbf{Ours (VoxCNN + XGA)}} & \text{0.9252} $\pm$ \text{0.054} &\text{0.9186} $\pm$ \text{0.036} & \text{0.8953} $\pm$ \text{0.053} & \text{0.9112} $\pm$ \text{0.073} \\

\bottomrule
\end{tabular}
\end{table*}

%%%%%%%%%%%%%%%%%%%%%%%%%%%%%%%%%%%%%%%%%%%%%%%%%%%%%%%
\clearpage
\section*{Section 4: Qualitative Results of the Interpolation}
\label{sup:4interpolation}
\begin{figure}[h]
    \centering\includegraphics[scale=0.11]{TPAMI2021-draft-his-0720/}
    \caption{Example of counterfactual map conditioned on interpolated target labels (Subject ID 123\_S\_0106, Image ID on top left corner). The purple and green boxes correspond to the ventricular and cortex regions, respectively. Parentheses $\{\cdot\}$ and $[\cdot]$ for condition indicate the posterior probability and a target label, respectively.}
    \label{fig:sup3interpolation}
\end{figure}

%%%%%%%%%%%%%%%%%%%%%%%%%%%%%%%%%%%%%%%%%%%%%%%%%%%%%%%

\section*{Section 5: Effectiveness of XGA and Guidance Maps}\label{sup:5effect}

To verify the effectiveness of the XGA module and guidance map in our framework, we performed ablation studies among the proposed method and the existing attention-based approaches~\cite{hu2018squeeze,linsley2018learning}. The validity of the proposed method was verified by providing the explicit significance of the derived performance using the Wilcoxon signed-rank test. Furthermore, we showed performance variations through self-iterative training of CMG and XGA modules.

Here, we benchmark the proposed XGA module against existing attention-based approaches, including squeeze-and-excitation (SE)~\cite{hu2018squeeze} and global-and-local attention (GALA)~\cite{linsley2018learning} on the ResNet18~\cite{he2016deep} architecture. Furthermore, to validate the effectiveness of the guidance map, the results were analyzed through the experimental setup with and without guidance maps in all scenarios (Table~\ref{table:ablation_attention}).
% All settings using a guidance map are calculated with the attention mask $\mathbf{A}$ of the XGA module injected into the first convolution block.
The results of our LEAR framework are significantly better than those of all other attention-based approaches. It should be noted that the additive dilated convolutions in the XGA module are also compatible with the aforementioned approaches. The most notable gains in performance were achieved when guidance maps were used to supervise our XGA module. We also conducted a Wilcoxon signed-rank test to validate the effectiveness of our proposed method and found that it demonstrated statistical significance as compared with the other methods, with $p$-values of 0.05 and 0.05 for the ACC and mAUC, respectively.

\begin{table}[h]\scriptsize \setlength{\tabcolsep}{5pt}
    \centering
    \caption{Effectiveness of our proposed XGA module and the guidance map on ADNI dataset. $*$ denotes the statistical significance in $p<0.05$.}
    \label{table:ablation_attention}
    \begin{tabular}{cccc}
    \toprule
   \multicolumn{1}{c}{\textbf{Guidance}}&\multicolumn{1}{c}{\textbf{Methods}} & \multicolumn{1}{c}{\textbf{mAUC}} & \multicolumn{1}{c}{\textbf{ACC}}\\
\midrule
    &SE~\cite{hu2018squeeze}&\multicolumn{1}{c}{\text{0.7558} $\pm$ \text{0.056}}&\multicolumn{1}{c}{\text{0.5791} $\pm$ \text{0.047}}\\
    &GALA~\cite{linsley2018learning}&\multicolumn{1}{c}{\text{0.7642} $\pm$ \text{0.061}} &\multicolumn{1}{c}{\text{0.5824} $\pm$ \text{0.038}}\\
    &\textbf{ResNet18 + XGA}&\multicolumn{1}{c}{\enspace\text{0.7827} $\pm$ \text{0.049}$^*$} &\multicolumn{1}{c}{\enspace\textbf{0.6491} $\pm$ \textbf{0.058}$^*$}\\
    &\textbf{SonoNet16 + XGA}&\multicolumn{1}{c}{\enspace\textbf{0.7892} $\pm$ \textbf{0.053}$^*$} &\multicolumn{1}{c}{\enspace\text{0.6381} $\pm$ \text{0.037}$^*$}\\
    &\textbf{VoxCNN + XGA}&\multicolumn{1}{c}{\text{0.7821} $\pm$ \text{0.054}} &\multicolumn{1}{c}{\enspace\text{0.6398} $\pm$ \text{0.052}$^*$}\\
    
    \cmidrule(lr){1-4}
    \hspace{0.cm}\parbox[t]{2mm}{\multirow{5}{*}{\rotatebox[origin=c]{0}{$\checkmark$}}}&SE~\cite{hu2018squeeze}&\multicolumn{1}{c}{\text{0.7683} $\pm$ \text{0.052}} &\multicolumn{1}{c}{\text{0.6231} $\pm$ \text{0.055}}\\
    &GALA~\cite{linsley2018learning}&\multicolumn{1}{c}{\text{0.7696} $\pm$ \text{0.067}} &\multicolumn{1}{c}{\text{0.6302} $\pm$ \text{0.048}}\\
    &\textbf{ResNet18 + XGA}&\multicolumn{1}{c}{\enspace\textbf{0.8123} $\pm$ \textbf{0.052}$^*$} &\multicolumn{1}{c}{\enspace\textbf{0.6715} $\pm$ \textbf{0.051}$^*$}\\
    &\textbf{SonoNet16 + XGA}&\multicolumn{1}{c}{\enspace\text{0.8085} $\pm$ \text{0.061}$^*$} &\multicolumn{1}{c}{\enspace\text{0.6689} $\pm$ \text{0.048}$^*$}\\
    &\textbf{VoxCNN + XGA}&\multicolumn{1}{c}{\enspace\text{0.8021} $\pm$ \text{0.062}$^*$} &\multicolumn{1}{c}{\enspace\text{0.6528} $\pm$ \text{0.044}$^*$}\\
\bottomrule
\end{tabular}
\end{table}

\clearpage
\section*{Section 6. Iterative learning scheme to various backbone diagnostic models}\label{sup:6iter}
\begin{figure}[h]
    \centering
    \includegraphics[scale=0.1]{TPAMI2021-draft-his-0720/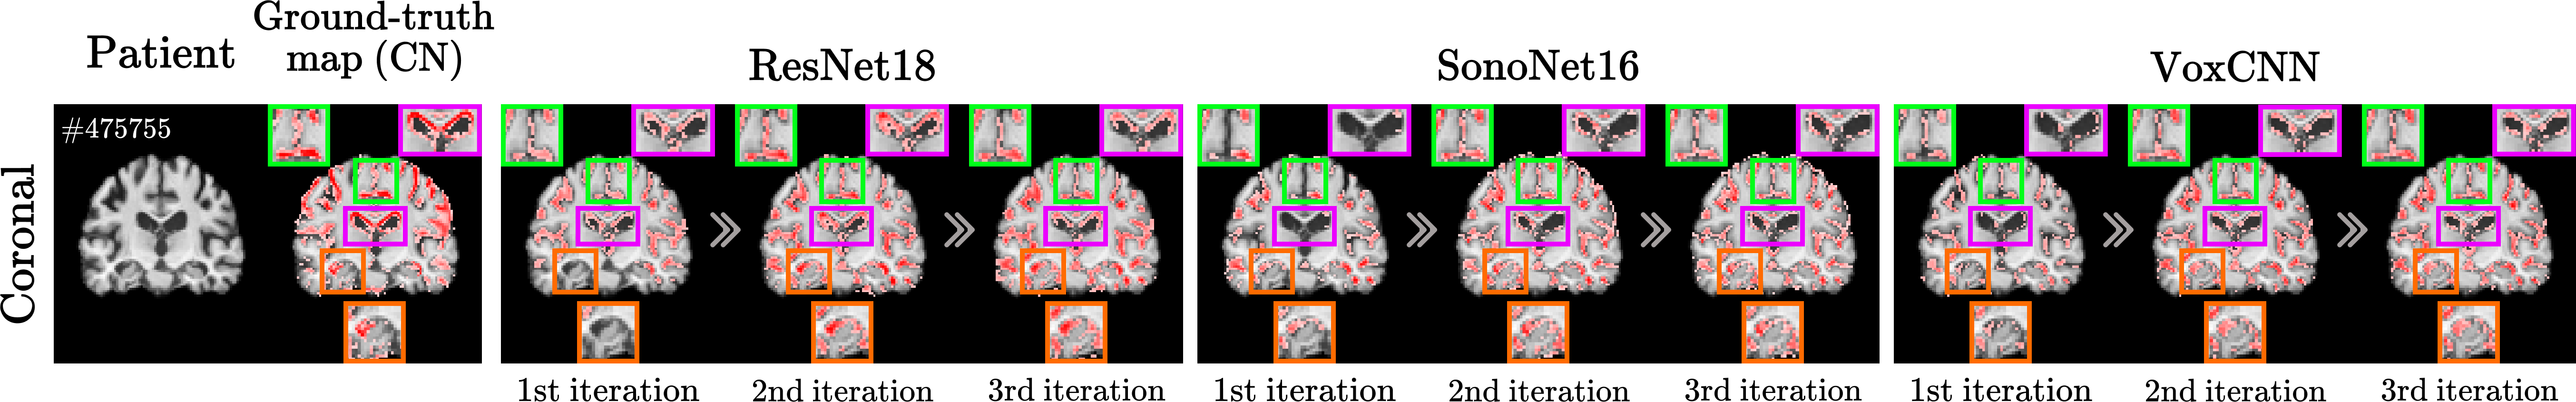}
    \caption{Reinforced counterfactual map visualization in various diagnostic models via iterative learning scheme (Subject ID 131\_S\_0123, Image ID on top left corner). The purple, orange, and green boxes correspond to the ventricular, hippocampus, and cortex regions, respectively.}
    \label{fig:iterative_3net}
\end{figure}

%%%%%%%%%%%%%%%%%%%%%%%%%%%%%%%%%%%%%%%%%%%%%%%%%%%%%%%%%%%%%%%%
